# Supplementary material for: Fast, Scalable Approximations to Posterior Distributions in Extended Latent Gaussian Models
Source: arXiv:2103.07425 source file (2022-07-12)
Supplement: Supplementary file 1 [file appendix-proof-v2.tex]

%!TEX root = ../main.tex

\section{Proof of Theorem \ref{thm:convergence}}\label{appendix:proof}

\subsection{Definitions}

For $n\in\N$, let $\truemeasuren$ denote the probability measure generating $\data\in\R^{n}$. For $\pi(\paramfullflip,\data) = \pi(\data|\parambig,\paramsmall_{1})\pi(\parambig|\paramsmall_{2})\pi(\paramsmall)$, let $\jointmode = \text{argmax}_{\paramfull}\log\pi(\paramfullflip,\data)$, and $$\truehess(\paramfull) = -\partial^{2}_{\paramfull}\log\pi(\paramfullflip,\data) \equiv \begin{pmatrix} \truehesssmall(\paramfull) & \truehessmixed(\paramfull) \\ \truehessmixedt(\paramfull) & \truehessbig(\paramfull) \end{pmatrix},$$ having ordered eigenvalues $\eigen_{1}\left\{\truehess(\paramfull)\right\} \geq \cdots \geq \eigen_{\paramsmalldim+\Wdim}\left\{\truehess(\paramfull)\right\}$. Further, let $\truehess(\paramfull)\inv = \truechol(\paramfull)\truechol(\paramfull)\tpose$, where $$\truechol(\paramfull) \equiv \begin{pmatrix} \truecholsmall(\paramfull) & \cdot \\ \truecholmixed(\paramfull) & \truecholbig(\paramfull) \end{pmatrix}$$ is the lower Cholesky triangle. For $\epsilon>0,d\in\N$, and $\mb{x}^{*}\in\R^{d}$, let $$\ball{\epsilon}{\mb{x}^{*}} = \bracevec{\mb{x}\in\R^{d}:\Ltnorm{\mb{x} - \mb{x}^{*}} < \epsilon}\subset\R^{d}.$$ Further, define
\begin{equation}\begin{aligned}
\paramsmallmode(\parambig) =& \ \text{argmax}_{\paramsmall}\log\pi(\paramfullflip,\data), \\
\approxpiW(\parambig|\data) &= \abs{\truecholsmall\left\{\paramsmallmode(\parambig),\parambig\right\}}\sum_{\quadpoint\in\quadpointset(\paramsmalldim,\quadnum)}\pi\left[\parambig,\truecholsmall\left\{\paramsmallmode(\parambig),\parambig\right\}\quadpoint+\paramsmallmode(\parambig)|\data\right]\weight_{k}(\quadpoint), \\
\approxpiS(\parambig|\data) &= \abs{\laplacechol}\sum_{\quadpoint\in\quadpointset(\paramsmalldim,\quadnum)}\pi(\parambig,\laplacechol\quadpoint+\laplacemode|\data)\weight_{k}(\quadpoint).
\end{aligned}\end{equation}

\subsection{Regularity conditions}\label{app:proof:conditions}

There are a number of sufficient regularity conditions we assume on the model $\pi(\parambig,\paramsmall,\data)$. Because the approximation $\approxpi(\parambig|\data)$ depends on three component approximations, our regularity conditions come from three sources.

\subsubsection*{Adaptive Gauss-Hermite Quadrature}
\citet{aghq} analyze the asymptotic properties of Adaptive Gauss Hermite Quadrature, under standard regularity conditions \citep[Appendix A]{aghq} on the model. We assume the same conditions, which we repeat explicitly here. While we state them in terms of $(\paramfull)$, note that we assume throughout that equivalent conditions hold for each of the true marginal posteriors $\pi(\parambig|\data)$ and $\pi(\paramsmall|\data)$, as appropriate. 

We assume there exists $\universalradius>0$ and $\paramfulltrue\in\paramspacefull$ such that the following hold:
%Our proof of \cref{thm:mainresult} relies on the following assumptions.

\begin{assumption}\label{assn:kderiv}
There exists $\derivnum\geq4$ such that $\pi(\paramfullflip,\data)$ is $\derivnum$-times continuously differentiable as a function of $(\paramfullflip)$, and $\derivbound>0$ such that for all $\dumderivvec \subseteq \N^{\paramsmalldim+\Wdim}$ with $0 \leq \abs{\dumderivvec} \leq \derivnum$,
$$
	\lim_{n \to \infty} \truemeasuren\left\{\sup_{(\paramfull) \in \ball{\universalradius}{(\paramfulltrue)}}\abs{\partial^{\dumderivvec}\log\pi(\paramfull,\data)} < n \derivbound\right\}=1.
$$
\end{assumption}

\begin{assumption} \label{assn:hessian}
There exist $0 < \hesssmall \leq \hessbig < \infty$ such that 
%for large enough $n$, if $\param \in \ball{\paramdim}{\paramtrue}{\universalradius}$ then  
\*[
	\lim_{n \to \infty} \truemeasuren\left[n \hesssmall \leq \inf_{(\paramfull) \in \ball{\universalradius}{(\paramfulltrue)}}\eigen_{\paramsmalldim+\Wdim}\left\{\truehess(\paramfull)\right\} \leq \sup_{(\paramfull) \in \ball{\universalradius}{(\paramfulltrue)}} \eigen_{1}\left\{\truehess(\paramfull)\right\}  \leq n \hessbig\right] = 1.
\]
\end{assumption}

\begin{assumption}\label{assn:limsup}
There exists $\llhoodmargin>0$ such that 
\*[
	\lim_{n \to \infty} \truemeasuren\left\{\sup_{(\paramfull) \in \ballc{\universalradius}{(\paramfulltrue)}} \log\pi(\data|\parambig,\paramsmall_{1}) - \log\pi(\data|\parambig_{0},\paramsmall_{0}) \leq -n \llhoodmargin\right\} = 1.
\]
\end{assumption}

\begin{assumption}\label{assn:consistency}
For any $\conmargin > 0$ and function $G(n)$ such that $\lim_{n \to \infty} G(n) = \infty$,
\*[
  \lim_{n \to \infty} \truemeasuren \left\{ \frac{n^{1/2}}{G(n)} \Ltnorm{\jointmode - (\paramfulltrue)} < \conmargin \right\} = 1.
\]
% There exists $\conmargin > 0$ such that
% \*[
%   \lim_{n \to \infty} \truemeasuren \left[ n^{1/2} \Ltnorm{\jointmode - (\paramfulltrue)} < \conmargin \right] = 1.
% \]
\end{assumption}

\begin{assumption}\label{assn:prior}
There exist  $0 < \priorsmall < \priorbig < \infty$ such that
\*[
   \priorsmall \leq \inf_{(\paramfull) \in \ball{\universalradius}{(\paramfulltrue)}} \pi(\paramfull) \leq \sup_{(\paramfull) \in \ball{\universalradius}{(\paramfulltrue)}} \pi(\paramfull) \leq \priorbig.
\]
\end{assumption}

Assumptions \ref{assn:kderiv} and \ref{assn:hessian} hold for conditionally independent likleihoods (\S\ref{subsec:elgms:definition}) where each individual likelihood contribution has $m\geq4$ uniformly bounded derivatives. Assumption \ref{assn:limsup} is asymptotic local identifiability of the ``true'' concentration point $(\paramfulltrue)$, which can be regarded as a minimal assumption for inference. Assumption \ref{assn:consistency} is consistency of the posterior mode, and Assumption \ref{assn:prior} states that the prior cannot exclude $(\paramfulltrue)$.

\subsubsection*{Gaussian Approximation}

For each $\paramsmalldim\in\N,\quadnum\in\N,\quadpoint\in\quadpointset(\paramsmalldim,\quadnum)$, we require a Bernstein von-Mises (BvM) theorem for $\gaussapprox(\parambig|\data,\laplacechol\quadpoint+\laplacemode)$, specifically, that there exists $C>0$ such that
\begin{equation}\label{eqn:bvmconditional}
\lim_{n\to\infty}\truemeasuren\left(\tvnorm{\pi(\parambig|\data,\laplacechol\quadpoint+\laplacemode) - \gaussapprox(\parambig|\data,\laplacechol\quadpoint+\laplacemode)} < Cn^{-1/2}\right) = 1.
\end{equation}
This is not a trivial application of the ``ordinary'' BvM theorem (e.g. \citealt[Ch. 10.2]{vandervaart}), because evaluating the conditional density at $\laplacechol\quadpoint+\laplacemode$ induces data-dependent misspecification, and violates any IID assumption for $\data$ (which we do not make in the first place). \citet[Thm. 2.1]{misspec} prove that this convergence holds under the stochastic Local Asymptotic Normality condition, which we state here as Assumption \ref{ass:lan} \citep[Eq. 2.1]{misspec}:
\begin{assumption}\label{ass:lan}
For each $\paramsmalldim\in\N,\quadnum\in\N$ there exists random vectors $\lanrandomvec$, bounded in probability, and non-singular matrices $\lanmat$ such that for every compact $\lanset\subset\R^{\Wdim+\paramsmalldim}$ and $\conmargin>0$:
$$
\lim_{n\to\infty}\truemeasuren\left\{\sup_{\lanvec\in\lanset}\abs{\log\frac{\pi(\data|(\paramfulltrue) + n^{-1/2}\lanvec)}{\pi(\data|\paramfulltrue)} - \lanvec\tpose\lanmat\lanrandomvec - \frac{1}{2}\lanvec\tpose\lanmat\lanvec} < \conmargin\right\} = 1.
$$
\end{assumption}

\subsubsection*{Laplace Approximation}

We require conditions on the model such that for any $\epsilon>0$,
\begin{equation}\begin{aligned}\label{eqn:laplaceconvergence}
\lim_{n\to\infty}\truemeasuren\left(n^{1/2}\Ltnorm{\laplacemode - \paramsmallmode} < \epsilon\right) = 1, \\
\lim_{n\to\infty}\truemeasuren\left(n^{-1}\Ltnorm{\laplacehess - \truehesssmall\jointmode} < \epsilon\right) = 1. \\
\end{aligned}\end{equation}
Note that this also implies that Assumptions 1 -- 5 hold for $\laplaceapprox(\paramsmall,\data)$. \citet[Lemma 1/Theorem 2]{approximatelikelihood} gives sufficient conditions, which we state here as Assumption \ref{ass:laplacescore}:
\begin{assumption}\label{ass:laplacescore}
For every $\epsilon>0$ , $$\lim_{n\to\infty}\truemeasuren\left( n^{-1}\sup_{\paramsmall\in\R^{\paramsmalldim}}\Ltnorm{\partial_{\paramsmall}\log\pi(\paramsmall,\data) - \partial_{\paramsmall}\laplaceapprox(\paramsmall,\data)} < \epsilon \right) = 1.$$ Further, there exists $t>0$ such that $$\lim_{n\to\infty}\truemeasuren\left( n^{-1/2}\sup_{\paramsmall\in\ball{t}{\paramsmalltrue}}\Ltnorm{\partial_{\paramsmall}\log\pi(\paramsmall,\data) - \partial_{\paramsmall}\laplaceapprox(\paramsmall,\data)} < \epsilon \right) = 1.$$
\end{assumption}

\subsection{Preliminary Lemmas}\label{app:proof:prelims}

We state the following preliminary Lemmas, all under Assumptions 1 -- \ref{ass:laplacescore}.

\begin{lemma}\label{lem:cholconvergence}
There exists $C>0$ such that $$\lim_{n\to\infty}\truemeasuren\left(\abs{\laplacechol} < Cn^{-\paramsmalldim/2} \right) = 1.$$
\end{lemma}
\begin{proof}
Under Assumption \ref{ass:laplacescore}, Assumptions \ref{assn:kderiv} -- \ref{assn:prior} hold for $\laplaceapprox(\paramsmall,\data)$. Since $\abs{\laplacechol} = \prod_{j=1}^{\paramsmalldim}\eigen_{j}\left\{\laplacehess(\laplacemode)\right\}^{-1/2}$ almost surely for any $n\in\N$, it follows from Assumption \ref{assn:hessian} that
$$
\lim_{n\to\infty}\truemeasuren\left(\abs{\laplacechol} < Cn^{-\paramsmalldim/2} \right)
= \lim_{n\to\infty}\truemeasuren\left[\prod_{j=1}^{\paramsmalldim}\eigen_{j}\left\{\laplacehess(\laplacemode)\right\}^{-1/2} < Cn^{-\paramsmalldim/2} \right] = 1,
$$
with $C = \hesssmall^{-\paramsmalldim/2}$.
\end{proof}

The proofs of Lemmas \ref{lem:insideball} and \ref{lem:outsideball} are more involved, and are given in Appendix \ref{app:proof:biglemmas}.
\begin{lemma}\label{lem:insideball}
For every $\epsilon>0$,
$$
\lim_{n\to\infty}\truemeasuren\left[\sup_{\borelset\in\borelsets{\paramsmalldim}}\sup_{\parambig\in\borelset\cap\ball{\universalradius}{\parambigtrue}}\abs{\frac{\approxpiS(\parambig|\data)}{\approxpiW(\parambig|\data)} - 1} < \epsilon\right] = 1.
$$
\end{lemma}

\begin{lemma}\label{lem:outsideball}
There exists $C>0$ such that
$$
\lim_{n\to\infty}\truemeasuren\left[\sup_{\borelset\in\borelsets{\paramsmalldim}}\abs{\int_{\borelset\cap\ballc{\paramfulltrue}{\universalradius}}
\pi(\parambig|\data) - \approxpiS(\parambig|\data)d\parambig} < Cn^{-1/2}\right].
$$
\end{lemma}

\subsection{Proof of Theorem \ref{thm:convergence}}\label{app:subsec:proof-theorem}

\setcounter{theorem}{0}
\begin{theorem}\label{thm:convergence}
Under Assumptions 1 -- \ref{ass:laplacescore} (Appendix \ref{app:proof:conditions}), $\tvnorm{\pi(\parambig|\data) - \approxpi(\parambig|\data)} = o_{p}(1).$
\end{theorem}
\begin{proof}
We wish to show that for every $\epsilon>0$,
$$\lim_{n\to\infty}\truemeasuren\left(\tvnorm{\pi(\parambig|\data) - \approxpi(\parambig|\data)} < \epsilon\right) = 1.$$
We split the total variation error into three terms which quantify the error induced by each of the three component approximations. By the triangle inequality,
\begin{equation}\begin{aligned}
&\sup_{\borelset\in\borelsets{\Wdim}}\abs{\int_{\borelset}\pi(\parambig|\data) - \approxpi(\parambig|\data)d\parambig} \\ 
\leq 
&\abs{\laplacechol}\sum_{\quadpoint\in\quadpointset(\paramsmalldim,\quadnum)}\sup_{\borelset(\quadpoint)\in\borelsets{\Wdim}}\abs{\int_{\borelset(\quadpoint)} \left\{\gaussapprox(\parambig|\data,\laplacechol\quadpoint+\laplacemode) - \pi(\parambig|\data,\laplacechol\quadpoint+\laplacemode)\right\}d\parambig}\laplaceapprox(\laplacechol\quadpoint+\laplacemode|\data)\weight_{k}(\quadpoint)\\
& + \abs{\laplacechol}\sum_{\quadpoint\in\quadpointset(\paramsmalldim,\quadnum)}\sup_{\borelset(\quadpoint)\in\borelsets{\Wdim}}
\abs{\int_{\borelset(\quadpoint)}
\pi(\parambig|\data,\laplacechol\quadpoint+\laplacemode)d\mb{W}}\pi(\laplacechol\quadpoint+\laplacemode|\data)
\left\{
\frac{\laplaceapprox(\laplacechol\quadpoint+\laplacemode|\data)}{\pi(\laplacechol\quadpoint+\laplacemode|\data)} - 1 \right\}\weight_{k}(\quadpoint)\\
& + \sup_{\borelset\in\borelsets{\Wdim}}
\abs{\int_{\borelset}
\pi(\parambig|\data) - \abs{\laplacechol}\sum_{\quadpoint\in\quadpointset(\paramsmalldim,\quadnum)}\pi(\parambig,\laplacechol\quadpoint+\laplacemode|\data)\weight_{k}(\quadpoint)d\parambig.
}\\
\end{aligned}\end{equation}
Lemma \ref{lem:gaussian} shows that the first term is $O_{p}(n^{-1/2})$, Lemma \ref{lem:laplace} shows that the second term is $O_{p}(n^{-\paramsmalldim/2})$, and Lemma \ref{lem:quadconvergence} shows that the third term is $o_{p}(1)$, which completes the proof of Theorem \ref{thm:convergence}.
\end{proof}

The remainder of this Appendix is devoted to proving Lemmas \ref{lem:gaussian}, \ref{lem:laplace}, and \ref{lem:quadconvergence}.

\subsection{Helper Lemmas}\label{app:proof:lemmas}

The following Lemmas hold under Assumptions 1 -- \ref{ass:laplacescore}.

\begin{lemma}\label{lem:gaussian}
There exists $C>0$ such that 
\begin{equation*}\begin{aligned}
\lim_{n\to\infty}\truemeasuren\Big[ &\abs{\laplacechol}\sum_{\quadpoint\in\quadpointset(\paramsmalldim,\quadnum)}\sup_{\borelset(\quadpoint)\in\borelsets{\Wdim}}  
\abs{\int_{\borelset(\quadpoint)} \left\{\gaussapprox(\parambig|\data,\laplacechol\quadpoint+\laplacemode) - \pi(\parambig|\data,\laplacechol\quadpoint+\laplacemode)\right\}d\parambig} \times \\
&\laplaceapprox(\laplacechol\quadpoint+\laplacemode|\data)\weight_{k}(\quadpoint) < Cn^{-1/2}\Big] = 1.
\end{aligned}\end{equation*}
\end{lemma}
\begin{proof}
By Assumption \ref{ass:lan}, there exists a $C>0$ such that $$\lim_{n\to\infty}\truemeasuren\left\{\max_{\quadpoint\in\quadpointset(\paramsmalldim,\quadnum)}\sup_{\borelset(\quadpoint)\in\borelsets{\Wdim}}\abs{\int_{\borelset(\quadpoint)}\pi(\parambig|\data,\laplacechol\quadpoint+\laplacemode) - \gaussapprox(\parambig|\data,\laplacechol\quadpoint+\laplacemode)} < Cn^{-1/2}\right\} = 1.$$ Equation (\ref{eqn:laplace}) implies that for all $n\in\N$, $$\truemeasuren\left\{ \abs{\laplacechol}\sum_{\quadpoint\in\quadpointset(\paramsmalldim,\quadnum)}\laplaceapprox(\laplacechol\quadpoint+\laplacemode|\data)\weight_{k}(\quadpoint) = 1 \right\} = 1.$$ Lemma \ref{lem:gaussian} follows immediately.
\end{proof}

\begin{lemma}\label{lem:laplace}
There exists $C>0$ such that
\begin{equation*}\begin{aligned}
\lim_{n\to\infty}\truemeasuren\Big[ &\abs{\laplacechol}\sum_{\quadpoint\in\quadpointset(\paramsmalldim,\quadnum)}\sup_{\borelset(\quadpoint)\in\borelsets{\Wdim}}\abs{\int_{\borelset(\quadpoint)}
\pi(\parambig|\data,\laplacechol\quadpoint+\laplacemode)d\mb{W}} \\
&\pi(\laplacechol\quadpoint+\laplacemode|\data)
\left\{
\frac{\laplaceapprox(\laplacechol\quadpoint+\laplacemode|\data)}{\pi(\laplacechol\quadpoint+\laplacemode|\data)} - 1 \right\}\weight_{k}(\quadpoint) < Cn^{-\paramsmalldim/2} \Big] = 1.
\end{aligned}\end{equation*}
\end{lemma}
\begin{proof}
For any $n\in\N$, $$\truemeasuren\left\{\max_{\quadpoint\in\quadpointset(\paramsmalldim,\quadnum)}\sup_{\borelset(\quadpoint)\in\borelsets{\Wdim}}\abs{\int_{\borelset(\quadpoint)}\pi(\parambig|\data,\laplacechol\quadpoint+\laplacemode)d\mb{W}} = 1 \right\} = 1.$$ \citet{validitylaplace} show that there exists $C_{1}>0$ such that 
\begin{equation}\label{eqn:kasslaplace}
\lim_{n\to\infty}\truemeasuren\left\{\sup_{\paramsmall\in\R^{\paramsmalldim}}\abs{\frac{\laplaceapprox(\paramsmall|\data)}{\pi(\paramsmall|\data)} - 1} < C_{1}n^{-1}\right\} = 1,
\end{equation}
and \citet[Theorem 1]{aghq} confirms that this holds under Assumptions \ref{assn:kderiv} -- \ref{assn:prior}. Note that $\abs{\sum_{\quadpoint\in\quadpointset(\paramsmalldim,\quadnum)}\weight_{k}(\quadpoint)} < \infty$ for every $\paramsmalldim,\quadnum\in\N$. Now, applying Assumption \ref{assn:kderiv} with $\dumderivvec=\zero$, and Lemma \ref{lem:cholconvergence}, we may find $C_{2}>0$ such that $$ \lim_{n\to\infty}\truemeasuren\left\{ \abs{\laplacechol}\sum_{\quadpoint\in\quadpointset(\paramsmalldim,\quadnum)}\pi(\laplacechol\quadpoint+\laplacemode|\data)\weight_{k}(\quadpoint) < C_{2}n^{1-\paramsmalldim/2}\right\} = 1.$$ Combining these statements yields Lemma \ref{lem:laplace}.
\end{proof}

\begin{lemma}\label{lem:quadconvergence}
For every $\epsilon>0$, $$\lim_{n\to\infty}\truemeasuren\left\{ \sup_{\borelset\in\borelsets{\Wdim}}
\abs{\int_{\borelset}
\pi(\parambig|\data) - \abs{\laplacechol}\sum_{\quadpoint\in\quadpointset(\paramsmalldim,\quadnum)}\pi(\parambig,\laplacechol\quadpoint+\laplacemode|\data)\weight_{k}(\quadpoint)d\parambig.
} < \epsilon\right\} = 1.$$
\end{lemma}

\begin{proof}
The proof of Lemma \ref{lem:quadconvergence} is more involved than the previous Lemmas, and the heavy lifting is done using two further lemmas proved in \S\ref{app:proof:biglemmas}. We begin by splitting up the region of integration. For any $\borelset\in\borelsets{\Wdim}$, we have
\begin{equation*}\begin{aligned}
\abs{\int_{\borelset}
\pi(\parambig|\data) - \approxpiS(\parambig|\data)d\parambig} 
\leq& \ \abs{\int_{\borelset\cap\ball{\universalradius}{(\paramfulltrue)}}
\pi(\parambig|\data) - \approxpiS(\parambig|\data) d\parambig} \\
&+ \ \abs{\int_{\borelset\cap\ballc{\universalradius}{(\paramfulltrue)}}
\pi(\parambig|\data) - \approxpiS(\parambig|\data)d\parambig}.
\end{aligned}\end{equation*}
Lemma \ref{lem:outsideball} states that, for some $C>0$,
$$
\lim_{n\to\infty}\truemeasuren\left\{ \abs{\int_{\borelset\cap\ballc{\universalradius}{(\paramfulltrue)}}
\pi(\parambig|\data) - \approxpiS(\parambig|\data)d\parambig} < Cn^{-1/2}\right\} = 1.
$$
Further write:
$$
\abs{\int_{\borelset\cap\ball{\universalradius}{(\paramfulltrue)}}
\pi(\parambig|\data) - \approxpiS(\parambig|\data) d\parambig} = \abs{\int_{\borelset\cap\ball{\universalradius}{(\paramfulltrue)}}
\pi(\parambig|\data) - \approxpiW(\parambig|\data)\left\{\frac{\approxpiS(\parambig|\data)}{\approxpiW(\parambig|\data)}\right\} d\parambig} 
$$
It is a straightforward application of \citet[Theorem. 1]{aghq} to conclude that there exists $C>0$ such that
$$
\lim_{n\to\infty}\truemeasuren\left\{ \sup_{\borelset\in\borelsets{\Wdim}}
\abs{\int_{\borelset}
\pi(\parambig|\data) - \approxpiW(\parambig|\data)d\parambig} < Cn^{-\lfloor (k+2)/3\rfloor}\right\} = 1.
$$
Lemma \ref{lem:insideball} states that, for every $\epsilon>0$,
$$
\lim_{n\to\infty}\truemeasuren\left\{\sup_{\borelset\in\borelsets{\Wdim}}\sup_{\parambig\in\borelset\cap\ball{\universalradius}{(\paramfulltrue)}}\abs{\frac{\approxpiS(\parambig|\data)}{\approxpiW(\parambig|\data)} - 1} < \epsilon\right\} = 1,
$$
which completes the proof of Lemma \ref{lem:quadconvergence}.
\end{proof}

\subsection{Proof of Lemmas \ref{lem:insideball} and \ref{lem:outsideball}}\label{app:proof:biglemmas}

\subsubsection{Proof of Lemma \ref{lem:insideball}}

First, observe that \citep[Ch. 4.6]{profile}:
$$
\partial_{\parambig}\paramsmallmode(\parambig) = -\left\{\truehesssmall[\paramsmallmode(\parambig),\parambig]\right\}\inv\truehessmixedt[\paramsmallmode(\parambig),\parambig],
$$
where the matrices on the RHS are continuous in $\parambig$ by Assumption \ref{assn:kderiv}. Since $\paramsmallmode(\parambig)$ is continuously differentiable, it is locally Lipschitz, and we conclude that there exists some $\universalradius \equiv \universalradius(\parambigmode) > 0$ and $M_{0}\equiv M_{0}(\parambigmode)>0$ such that whenever $\parambig\in\ball{\parambigmode}{\universalradius}$, we have $$\Ltnorm{\paramsmallmode(\parambig) - \paramsmallmode(\parambigmode)} \leq M_{0}\Ltnorm{\parambig - \parambigmode} \leq M_{0}\universalradius.$$ We also have that $\paramsmallmode(\parambigmode) = \paramsmallmode$, and that both $\parambigmode$ and $\paramsmallmode$ are consistent. Therefore, in the remainder of the proof, we may assume $\paramsmallmode(\parambig)\in\ball{\paramsmallmode}{\universalradius}$ whenever $\parambig\in\ball{\parambigmode}{\universalradius}$, and that any $\paramsmall\in\ball{\paramsmallmode}{\universalradius}$ may be interchanged with $\paramsmall\in\ball{\paramsmalltrue}{\universalradius}$, and similarly for $\parambig$ and $(\paramfull)$, by taking $n$ large enough, which we do in the final limiting statements.

Fix arbitrary $\borelset\in\borelsets{\paramsmalldim}$, and $\parambig\in\borelset\cap\ball{\parambigtrue}{\universalradius}$. Write
\begin{equation*}\begin{aligned}
\frac{\approxpiS(\parambig|\data)}{\approxpiW(\parambig|\data)} &= \frac{\abs{\laplacechol}\sum_{\quadpoint\in\quadpointset(\paramsmalldim,\quadnum)}\pi(\parambig,\laplacechol\quadpoint+\laplacemode|\data)\weight_{k}(\quadpoint)}{\abs{\truecholsmall\left\{\paramsmallmode(\parambig),\parambig\right\}}\sum_{\quadpoint\in\quadpointset(\paramsmalldim,\quadnum)}\pi\left[\parambig,\truecholsmall\left\{\paramsmallmode(\parambig),\parambig\right\}\quadpoint+\paramsmallmode(\parambig)|\data\right]\weight_{k}(\quadpoint)} \\
&\leq \frac{\abs{\laplacechol}}{\abs{\truecholsmall\left\{\paramsmallmode(\parambig),\parambig\right\}}}\sum_{\quadpoint\in\quadpointset(\paramsmalldim,\quadnum)}\frac{\pi(\parambig,\laplacechol\quadpoint+\laplacemode|\data)}{\pi\left[\parambig,\truecholsmall\left\{\paramsmallmode(\parambig),\parambig\right\}\quadpoint+\paramsmallmode(\parambig)|\data\right]}, 
\end{aligned}\end{equation*}
since for any $a,b,c,d > 0, (a+b)/(c+d) \leq a/b + c/d$. 

For the ratio of determinants, apply Assumption \ref{ass:laplacescore} to conclude that, for any $\epsilon>0$,
$$
\lim_{n\to\infty}\truemeasuren\left[ \sup_{\parambig\in\ball{\Wmode}{\universalradius}}\abs{ \abs{n^{1/2}\laplacechol} - \abs{n^{1/2}\truecholsmall\left\{\paramsmallmode(\parambig),\parambig\right\}}} < \epsilon\right] = 1.
$$
We have, for any $\parambig\in\ball{\Wmode}{\universalradius}$,
\begin{equation}\begin{aligned}
\abs{ \abs{n^{1/2}\laplacechol} - \abs{n^{1/2}\truecholsmall(\paramsmallmode(\parambig),\parambig)}} 
&= n^{\paramsmalldim/2}\abs{\laplacechol}\abs{\frac{\abs{\laplacechol}}{\abs{\truecholsmall\left\{\paramsmallmode(\parambig),\parambig\right\}}} - 1} \\
&\geq \hessbig^{-\paramsmalldim/2}\abs{\frac{\abs{\laplacechol}}{\abs{\truecholsmall\left\{\paramsmallmode(\parambig),\parambig\right\}}} - 1},
\end{aligned}\end{equation}
where the last line uses Assumption \ref{assn:hessian}. Conclude that for any $\epsilon>0$,
\begin{equation}\label{eqn:cholconvergence}
\lim_{n\to\infty}\truemeasuren\left[ \sup_{\parambig\in\ball{\Wmode}{\universalradius}}\abs{\frac{\abs{\laplacechol}}{\abs{\truecholsmall\left\{\paramsmallmode(\parambig),\parambig\right\}}}-1} < \hessbig^{\paramsmalldim/2}\epsilon\right] = 1.
\end{equation}
For the ratio of posteriors, fix arbitrary $\paramsmalldim,\quadnum\in\N,\quadpoint\in\quadpointset(\paramsmalldim,\quadnum)$, and $\parambig\in\ball{\Wmode}{\universalradius}$, and consider a third-order Taylor expansion of the log-ratio:
\begin{equation*}\begin{aligned}
&\log\pi\left(\parambig,\laplacechol\quadpoint+\laplacemode|\data\right) - \log\pi\left[\parambig,\truecholsmall\left\{\paramsmallmode(\parambig),\parambig\right\}\quadpoint+\paramsmallmode(\parambig)|\data\right] \\
=& -\frac{1}{2}\left( \left[ \laplacechol - \truecholsmall\left\{\paramsmallmode\left(\parambig\right),\parambig\right\}\right]\quadpoint + \left\{\laplacemode - \paramsmallmode(\parambig)\right\}\right)\tpose\truehesssmall\left\{\paramsmallmode(\parambig),\parambig\right\} \\
&\qquad\left( \left[ \laplacechol - \truecholsmall\left\{\paramsmallmode\left(\parambig\right),\parambig\right\}\right]\quadpoint + \left\{\laplacemode - \paramsmallmode(\parambig)\right\}\right) + \\
&\frac{1}{6}\biggl( 
\left\{ \laplacechol\quadpoint + \laplacemode - \paramsmallmode(\parambig)\right\}_{i_{1}i_{2}i_{3}}\partial^{i_{1}i_{2}i_{3}}
\log\pi\left\{\parambig,\paramsmall^{*}_{1}(\parambig)\right\} - \\
&\qquad\left[ \truecholsmall\left\{\parambig,\paramsmallmode(\parambig)\right\}\quadpoint\right]_{i_{1}i_{2}i_{3}}\partial^{i_{1}i_{2}i_{3}}
\log\pi\left\{\parambig,\paramsmall^{*}_{2}(\parambig)\right\}\biggr),
\end{aligned}\end{equation*}
where $\paramsmall^{*}_{1}(\parambig) = t_{1}(\laplacechol\quadpoint+\laplacemode) + (1-t_{1})\paramsmallmode(\parambig)$ and $\paramsmall^{*}_{2}(\parambig) = t_{2}\truecholsmall\left\{\parambig,\paramsmallmode(\parambig)\right\}\quadpoint + \paramsmallmode(\parambig)$ for some $t_{1},t_{2}\in[0,1]$, and hence for $n$ large enough it will be the case (with high probability) that $\paramsmall^{*}_{j}(\parambig)\in\ball{\paramsmalltrue}{\universalradius}, j=1,2$.

For the third-order term, we bound the tensor products as
\begin{equation*}\begin{aligned}
\left\{ \laplacechol\quadpoint + \laplacemode - \paramsmallmode(\parambig)\right\}_{i_{1}i_{2}i_{3}} &\leq \paramsmalldim^{3}\left\{ \opnorm{\laplacechol}\Ltnorm{\quadpoint} + \Ltnorm{\laplacemode - \paramsmallmode(\parambig)}\right\}^{3}, \\
\left[ \truecholsmall\left\{\parambig,\paramsmallmode(\parambig)\right\}\quadpoint\right]_{i_{1}i_{2}i_{3}} &\leq \paramsmalldim^{3}\left[ \opnorm{\truecholsmall\left\{\parambig,\paramsmallmode(\parambig)\right\}}\Ltnorm{\quadpoint}\right]^{3}, \\
\partial^{i_{1}i_{2}i_{3}}
\log\pi\left\{\parambig,\paramsmall^{*}_{1}(\parambig)\right\} &\leq \paramsmalldim^{3}\max_{i_{1},i_{2},i_{3}\in[\paramsmalldim]}\partial^{i_{1}i_{2}i_{3}}\log\pi\left\{\parambig,\paramsmall^{*}_{1}(\parambig)\right\},
\end{aligned}\end{equation*}
and apply Assumptions \ref{assn:kderiv}, \ref{assn:hessian} and \ref{ass:laplacescore} to conclude that there exists some $C_{1},C_{2},C_{3}>0$ such that
\begin{equation*}\begin{aligned}
\lim_{n\to\infty}&\truemeasuren\left[ \left\{ \laplacechol\quadpoint + \laplacemode - \paramsmallmode(\parambig)\right\}_{i_{1}i_{2}i_{3}} < C_{1}n^{-3/2}\right] = 1, \\
\lim_{n\to\infty}&\truemeasuren\left( \left[ \truecholsmall\left\{\parambig,\paramsmallmode(\parambig)\right\}\quadpoint\right]_{i_{1}i_{2}i_{3}} < C_{2}n^{-3/2}\right) = 1, \\
\lim_{n\to\infty}&\truemeasuren\left[\partial^{i_{1}i_{2}i_{3}}
\log\pi\left\{\parambig,\paramsmall^{*}_{1}(\parambig)\right\} < C_{3}n\right] = 1.
\end{aligned}\end{equation*}
The second-order term limits the rate of convergence. We have, by Assumption \ref{ass:laplacescore} and Equation (\ref{eqn:laplaceconvergence}), for any $\epsilon>0$,
\begin{equation}\begin{aligned}
\lim_{n\to\infty}\truemeasuren\left(\sup_{\parambig\in\ball{\parambigmode}{\universalradius}}n^{1/2}\Ltnorm{\laplacemode - \paramsmallmode} < \epsilon\right) = 1, \\
\lim_{n\to\infty}\truemeasuren\left(\sup_{\parambig\in\ball{\parambigmode}{\universalradius}}n^{1/2}\Ltnorm{\laplacechol - \truecholsmall\left\{\paramsmallmode(\parambig),\parambig\right\}} < \epsilon\right) = 1.
\end{aligned}\end{equation}
Applying Assumption \ref{assn:hessian}, we therefore have for any $\epsilon>0$, with high probability as $n\to\infty$
\begin{equation}\begin{aligned}
&\left( \left[ \laplacechol - \truecholsmall\left\{\paramsmallmode\left(\parambig\right),\parambig\right\}\right]\quadpoint + \left\{\laplacemode - \paramsmallmode(\parambig)\right\}\right)\tpose\truehesssmall\left\{\paramsmallmode(\parambig),\parambig\right\} \\
&\qquad\left( \left[ \laplacechol - \truecholsmall\left\{\paramsmallmode\left(\parambig\right),\parambig\right\}\right]\quadpoint + \left\{\laplacemode - \paramsmallmode(\parambig)\right\}\right) \\
\leq& \ n\hessbig\left( \Ltnorm{\laplacechol - \truecholsmall\left\{\paramsmallmode\left(\parambig\right),\parambig\right\}}\Ltnorm{\quadpoint} + \Ltnorm{\laplacemode - \paramsmallmode(\parambig)} \right)^{2} \\
&\leq \ \hessbig\epsilon^{2}(\Ltnorm{\quadpoint}+1)^{2}.
\end{aligned}\end{equation}
Combining statements proves Lemma \ref{lem:insideball}.

\hfill$\square$

\subsubsection{Proof of Lemma \ref{lem:outsideball}}

Fix arbitrary $\borelset\in\borelsets{\Wdim}$. We argue separately that each term in the statement of Lemma \ref{lem:outsideball} is small. For the first term, write
\begin{equation*}\begin{aligned}
\int_{\borelset\cap\ballc{\universalradius}{\parambigtrue}}\pi(\parambig|\data)d\parambig &= \int_{\borelset\cap\ballc{\universalradius}{\parambigtrue}\times\R^{\paramsmalldim}}\pi(\parambig,\paramsmall|\data)d\parambig d\paramsmall \\
&= \int_{\borelset\cap\ballc{\universalradius}{\parambigtrue}\times\ball{\universalradius}{\paramsmalltrue}}\pi(\parambig,\paramsmall|\data)d\parambig d\paramsmall + \int_{\borelset\cap\ballc{\universalradius}{\parambigtrue}\times\ballc{\universalradius}{\paramsmalltrue}}\pi(\parambig,\paramsmall|\data)d\parambig d\paramsmall
\end{aligned}\end{equation*}
Using Assumptions \ref{assn:limsup} and \ref{assn:prior}, Lemma 6 from \citet[Appendix C.1]{aghq} states that
$$
\lim_{n\to\infty}\truemeasuren\left[ \int_{\ballc{\parambigtrue}{\universalradius}\times\ballc{\paramsmalltrue}{\universalradius}}\frac{\pi(\parambig,\paramsmall|\data)}{\pi(\parambigmode,\paramsmallmode|\data)}d\parambig d\paramsmall \leq \frac{e^{-nb}}{c_{1}}\right] = 1.
$$
Multiplying and dividing by $\pi(\parambigmode,\paramsmallmode|\data)$, and applying Assumption \ref{assn:kderiv}, we conclude that 
$$
\lim_{n\to\infty}\truemeasuren\left[ \int_{\ballc{\parambigtrue}{\universalradius}\times\ballc{\paramsmalltrue}{\universalradius}}\pi(\parambig,\paramsmall|\data)d\parambig d\paramsmall \leq Mn\frac{e^{-nb}}{c_{1}}\right] = 1.
$$
 
For the term where $\parambig$ is far from $\parambigtrue$ but $\paramsmall$ is close to $\paramsmalltrue$, we let the ordinary Bernstein von-Mises theorem (BvM; \citealt[Ch. 10.2]{vandervaart}) do the heavy lifting. Define a Gaussian approximation $\gaussapprox(\parambig,\paramsmall|\data)$ to $\pi(\parambig,\paramsmall|\data)$, and write
\begin{equation*}\begin{aligned}
&\int_{\borelset\cap\ballc{\universalradius}{\parambigtrue}\times\ball{\universalradius}{\paramsmalltrue}}\pi(\parambig,\paramsmall|\data)d\parambig d\paramsmall \\
=& \int_{\borelset\cap\ballc{\universalradius}{\parambigtrue}\times\ball{\universalradius}{\paramsmalltrue}}\pi(\parambig,\paramsmall|\data) -\gaussapprox(\parambig,\paramsmall|\data)d\parambig d\paramsmall 
+ \int_{\borelset\cap\ballc{\universalradius}{\parambigtrue}\times\ball{\universalradius}{\paramsmalltrue}}\gaussapprox(\parambig,\paramsmall|\data)d\parambig d\paramsmall
\end{aligned}\end{equation*}
We invoke BvM to conclude that for some $C>0$,
$$
\lim_{n\to\infty}\truemeasuren\left\{ \int_{\borelset\cap\ballc{\universalradius}{\parambigtrue}\times\ball{\universalradius}{\paramsmalltrue}}\pi(\parambig,\paramsmall|\data) -\gaussapprox(\parambig,\paramsmall|\data)d\parambig d\paramsmall < Cn^{-1/2}\right\} = 1.
$$
Further, we have
\begin{equation*}\begin{aligned}
&\int_{\borelset\cap\ballc{\universalradius}{\parambigtrue}\times\ball{\universalradius}{\paramsmalltrue}}\gaussapprox(\parambig,\paramsmall|\data)d\parambig d\paramsmall \\
=& \ (2\pi)^{-(\paramsmalldim+\Wdim)/2}\abs{\truehess\jointmode}^{1/2}\int_{\borelset\cap\ballc{\universalradius}{\parambigtrue}\times\ball{\universalradius}{\paramsmalltrue}}\exp\left\{ -\frac{1}{2}\begin{pmatrix}\paramsmall - \paramsmallmode \\ \parambig - \parambigmode \end{pmatrix}\tpose\truehess\jointmode\begin{pmatrix}\paramsmall - \paramsmallmode \\ \parambig - \parambigmode \end{pmatrix}\right\}d\paramsmall d\parambig \\
\leq& \ (2\pi)^{-(\paramsmalldim+\Wdim)/2} (\hesssmall n)^{(\paramsmalldim+\Wdim)/2}\int_{\borelset\cap\ballc{\universalradius}{\parambigtrue}}\exp\left\{ -\frac{\hesssmall n}{2}\Ltnorm{\parambig - \parambigmode}\right\}d\parambig\int_{\ball{\universalradius}{\paramsmalltrue}}\exp\left\{ -\frac{\hesssmall n}{2}\Ltnorm{\paramsmall - \paramsmallmode}\right\}d\paramsmall.
\end{aligned}\end{equation*}
The second term, an integral of a Gaussian around its mode, is bounded as
$$
\int_{\ball{\paramsmalltrue}{\universalradius}}\exp\left\{ -\frac{\hesssmall n}{2}\Ltnorm{\paramsmall - \paramsmallmode}\right\}d\paramsmall \leq (2\pi)^{\paramsmalldim/2}(\hesssmall n)^{-\paramsmalldim/2}.
$$
For the first term, a Gaussian tail integral, following the basic strategy of \citet[Lemma 7]{aghq}, we have
\begin{equation*}\begin{aligned}
\int_{\borelset\cap\ballc{\parambigtrue}{\universalradius}}\exp\left\{ -\frac{\hesssmall n}{2}\Ltnorm{\parambig - \parambigmode}\right\}d\parambig &= \left( \frac{2\pi}{\hesssmall n}\right)^{\Wdim/2} \PP\left\{ \chi^{2}_{\Wdim}/\Wdim \geq 1 + \left( \frac{\hesssmall n \universalradius^{2}}{\Wdim} - 1\right)\right\} \\
&\leq \left( \frac{2\pi}{\hesssmall n}\right)^{\Wdim/2}\exp\left[ \frac{\Wdim}{2}\left\{\log\left(\hesssmall n \universalradius^{2}\right) - \hesssmall n \universalradius^{2} + 1\right\}\right] \\
&\leq \left( \frac{2\pi e}{\hesssmall n}\right)^{\Wdim/2}\exp\left( -\frac{\hesssmall n \universalradius^{2}}{4}\right),
\end{aligned}\end{equation*}
where we have used $\log(x) < x/2$ for all $x\in\R$ and \citet[Lemma 3]{Fan}.

Combining all these statements, we have handled the first term: we have shown that there exists $C>0$ for which
$$
\lim_{n\to\infty}\truemeasuren\left\{ \sup_{\borelset\in\borelsets{\Wdim}}\int_{\borelset\cap\ballc{\universalradius}{\parambigtrue}}\pi(\parambig|\data)d\parambig < Cn^{-1/2}\right\} = 1.
$$
We turn now to the second term:
\begin{equation*}\begin{aligned}
\int_{\borelset\cap\ballc{\universalradius}{\parambigtrue}}\approxpiS(\parambig|\data)d\parambig &= \abs{\laplacechol}\sum_{\quadpoint\in\quadpointset(\paramsmalldim,\quadnum)}\int_{\borelset\cap\ballc{\universalradius}{\parambigtrue}}\pi(\parambig,\laplacechol\quadpoint+\laplacemode|\data)d\parambig\weight_{\quadnum}(\quadpoint). \\
% &\leq\abs{\laplacechol}\left\{\sum_{\quadpoint\in\quadpointset(\paramsmalldim,\quadnum)}\weight_{\quadnum}(\quadpoint)\right\}\int_{\borelset\cap\ballc{\universalradius}{\parambigtrue}}\pi(\parambig,\paramsmallmode|\data)d\parambig.
\end{aligned}\end{equation*}
Again rely on a Gaussian approximation,
\begin{equation*}\begin{aligned}
&\int_{\borelset\cap\ballc{\universalradius}{\parambigtrue}}\pi(\parambig,\laplacechol\quadpoint+\laplacemode|\data)d\parambig \\
= &\int_{\borelset\cap\ballc{\universalradius}{\parambigtrue}}\pi(\parambig,\laplacechol\quadpoint+\laplacemode|\data) - \gaussapprox(\parambig,\laplacechol\quadpoint+\laplacemode|\data)d\parambig \\
&+\int_{\borelset\cap\ballc{\universalradius}{\parambigtrue}}\gaussapprox(\parambig,\laplacechol\quadpoint+\laplacemode|\data)d\parambig,
\end{aligned}\end{equation*}
where we invoke Lemma \ref{lem:cholconvergence} along with the Bernstein von-Mises theorem again to conclude that, for some $C>0$,
$$
\lim_{n\to\infty}\truemeasuren\left\{\max_{\quadpoint\in\quadpointset(\paramsmalldim,\quadnum)}\sup_{\borelset\in\borelsets{\Wdim}} \abs{\laplacechol} \int_{\borelset\cap\ballc{\universalradius}{\parambigtrue}}\pi(\parambig,\laplacechol\quadpoint+\laplacemode|\data) - \gaussapprox(\parambig,\laplacechol\quadpoint+\laplacemode|\data)d\parambig < Cn^{-(s+1)/2}\right\} = 1.
$$
Following a similar strategy as above,
\begin{equation*}\begin{aligned}
&\int_{\borelset\cap\ballc{\universalradius}{\parambigtrue}}\gaussapprox(\parambig,\laplacechol\quadpoint+\laplacemode|\data)d\parambig \\
=& \ (2\pi)^{-(\paramsmalldim+\Wdim)/2} (\hesssmall n)^{(\paramsmalldim+\Wdim)/2}\int_{\borelset\cap\ballc{\universalradius}{\parambigtrue}}\exp\left( -\frac{\hesssmall n}{2}\Ltnorm{\parambig - \parambigmode}\right)d\parambig\cdot\exp\left(-\frac{\hesssmall n}{2}\Ltnorm{\laplacechol\quadpoint+\laplacemode - \paramsmallmode}\right) \\
&\leq (2\pi)^{-\paramsmalldim/2} (\hesssmall n)^{\paramsmalldim/2}e^{\Wdim/2}\exp\left( -\frac{\hesssmall n \universalradius^{2}}{4}\right),
\end{aligned}\end{equation*}
where we use the loose bound $\truemeasuren\left\{\exp\left(-\frac{\hesssmall n}{2}\Ltnorm{\laplacechol\quadpoint+\laplacemode - \paramsmallmode}\right) < 1 \right\}\to1$. Conclude that, again for some $C>0$,
\begin{equation*}\begin{aligned}
\lim_{n\to\infty}\truemeasuren\left\{\max_{\quadpoint\in\quadpointset(\paramsmalldim,\quadnum)}\sup_{\borelset\in\borelsets{\Wdim}} \abs{\laplacechol}\int_{\borelset\cap\ballc{\universalradius}{\parambigtrue}}\gaussapprox(\parambig,\paramsmallmode|\data)d\parambig < C\cdot(2\pi)^{-\paramsmalldim/2}e^{\Wdim/2}\exp\left( -\frac{\hesssmall n \universalradius^{2}}{4}\right)\right\} = 1.
\end{aligned}\end{equation*}

Combining these statements proves Lemma \ref{lem:outsideball}.

\hfill$\square$
